# Supplementary material for: Demographic Dialectal Variation in Social Media: A Case Study of African-American English
Source: arXiv:1608.08868 source file (2016-08-31)
Supplement: Supplementary file 1 [file appendix.tex]

\documentclass[11pt,letterpaper]{article}
%% alternative for ACL stylesheet
% \documentclass[11pt,a4paper]{article}
% \usepackage{acl2015}
% \usepackage{times}
% \usepackage[round]{natbib} % for ACL stylesheet: https://clear.colorado.edu/CompSemWiki/index.php/Adding_ACL_Style_Citations
\usepackage[top=1in,bottom=1in,left=1in,right=1in]{geometry}
\usepackage[round]{natbib} % for ACL stylesheet: 
\usepackage{palatino}
%\bibpunct{(}{)}{;}{a}{,}{,}
\usepackage{chngpage}
\usepackage{stmaryrd}
\usepackage{amssymb}
\usepackage{amsmath}
\usepackage{amsthm}
\usepackage{graphicx}
\usepackage{lscape}
\usepackage{subfigure}
\usepackage[usenames,dvipsnames]{color}
\definecolor{myblue}{rgb}{0,0.1,0.6}
\definecolor{mygreen}{rgb}{0,0.3,0.1}
\usepackage[colorlinks=true,linkcolor=black,citecolor=mygreen,urlcolor=myblue]{hyperref}
% possible colors: https://en.wikibooks.org/wiki/LaTeX/Colors#The_68_standard_colors_known_to_dvips

\newcommand{\ignore}[1]{}

\theoremstyle{definition}

\title{
Appendix for Demographic Dialectal Variation in Social Media:
A Case Study of African-American English}

\author{Su Lin Blodgett
    \ \  Lisa Green
    \ \ Brendan O'Connor \\
    University of Massachusetts Amherst
  }

%\date{December 9, 2009}

\begin{document}
\maketitle

\section{Appendix}

\input{appendix_body.tex}

\bibliographystyle{plainnat}
\bibliography{brenocon}
\end{document}
